# Supplementary material for: Value of Assistance for Grasping
Source: arXiv:2310.14402 source file (2024-03-18)
Supplement: Supplementary file 1 [file complexity.tex]

\subsection{Complexity Analysis}\label{sec:complexity}
%Exploring the complexity of algorithms is vital, it allows us to understand how the algorithm's performance scales with the size of the input or other relevant parameters. Additionally, analyzing the complexity can lead to insights for optimization and improvement, making the algorithm more efficient. As we analyze the steps of our algorithm, we'll keep an eye out for any parts that seem too slow or complicated. If we find these spots, we might be able to make them better.% We'll carefully go through the algorithm, step by step, to figure out its complexity, with the hope of finding ideas that might help improve it later on.

    We observe that $\estimatedSensorFunc\left(\helperConfig,\objPose\right)$ could be a bottleneck in the algorithm, depending on the sensor used. We will denote its complexity as $O(\alpha)$.

    \begin{enumerate}
        \item Outer Loop Over $\allObjStablePoses$: The outer loop iterates over the set of poses $\allObjStablePoses$, so it runs $|\allObjStablePoses|$ times.
        \item Observation Prediction Function and Belief Update: Within each iteration of the outer loop, the alpha function is called, adding $O(\alpha)$. The belief update is also called, which contains its own internal loop over $\allObjStablePoses$ and calls the alpha function in each iteration. Therefore, the belief update contributes $|\allObjStablePoses| \times O(\alpha)$.
        \item Grasp Calculation Over $\graspConfigSet$ and $\allObjStablePoses$: The best grasp calculation, which occurs for each pose, has a complexity of $|\graspConfigSet||\allObjStablePoses|$ since it runs for each grasp configuration and each pose.
    \end{enumerate}

    Combining the complexities from these components, we get:

    \begin{itemize}
        \item For each pose in $\allObjStablePoses$, the alpha function and the belief update yield $O(\alpha) + |\allObjStablePoses| \times O(\alpha)$.
        \item The grasp calculation contributes $|\graspConfigSet||\allObjStablePoses|$.
    \end{itemize}

    So the total complexity is given by: $|\allObjStablePoses| \times \left(O(\alpha) + |\allObjStablePoses| \times O(\alpha) + |\graspConfigSet||\allObjStablePoses|\right)$.

    Simplifying this expression, we get: $$O\left(|\allObjStablePoses|^2|\graspConfigSet|\right) + O\left(|\allObjStablePoses|^2 \times \alpha \right)$$

    our algorithm is developed for a specific sensor configuration $\helperConfig$. When we extend the algorithm to perform an $arg \max$ operation over a set of possible sensor configurations $\helperConfigs$ the time complexity becomes $O\left(|\helperConfigs|\times\left(|\allObjStablePoses|^2|\graspConfigSet| +|\allObjStablePoses|^2 \times \alpha \right)\right)$

    One significant optimization we've introduced involves the computation of $\alpha$ values, which are utilized at least $|P_o|$ times within the algorithm. Recognizing this, we precalculate the entire set of $\alpha$ values upfront. This strategic approach reduces the overall complexity from $O(|\allObjStablePoses|^2 \times \alpha)$ to $O(|\allObjStablePoses| \times \alpha)$. Subsequently, whenever an $\alpha$ value is needed, it can be retrieved in constant time, $O(1)$, significantly streamlining the algorithm's execution. However, it's important to note that this approach requires additional memory to store the precomputed observations values, thereby increasing the algorithm's space complexity. The overall time complexity is now $O\left(|\allObjStablePoses|^2|\graspConfigSet|\right) + O\left(|\allObjStablePoses| \times \alpha \right)$.

%Importantly, the \helper~and \actor~may not have the same belief or belief update function. %We therefore distinguish here between the belief of the 
\sk{TODO}

The \VOA~measure we develop here is based on the assumption that the agent that is performing its grasping task is equipped with one such methodology, and our aim it to account for the agent's policy in finding the best observation to support a successful grasping, our work is also strongly related to manipulation planning.
