# Supplementary material for: Value of Assistance for Grasping
Source: arXiv:2310.14402 source file (2024-03-18)
Supplement: Supplementary file 5 [file appendix-old.tex]

\section{Leftovers}

\subsection{Estimated Belief Update}
We define a distance metric between two observations 
% define distance function
\begin{definition}[Observation Similarity Metric]
Given two observations $\observation, \observation' \in \observations$, an {\em observation similarity metric} $\obsSimScore:\observations\times\observations\mapsto %\mathbb{R}_{\geq0}$
[0,1]$
associates a similarity score $\obsSimScore(\observation, \observation')$ between two observations.
\end{definition}



Here we assume that $\estimatedSensorFunc$ is deterministic and noiseless, such that the distance between two observations taken from the same sensor configurations (and the same sensing action) are the same and the distance between them is 0. 
%find a way to quantify how informative an observation is The observation that we get is
%$\observation_{\objPose,\sensingAction} = \estimatedSensorFunc\left({ \objPose, \sensingAction}\right)$
%The observation for object pose $\objPose'$ is
%$\observation_{\objPose',\sensingAction} = \estimatedSensorFunc\left({ \objPose', \sensingAction}\right)$


% \begin{equation}\label{eq:obsScore}
% \obsScore(\objPose_j,\estimatedObservation_{\objPose_i,\sensingAction})= \frac{1-\obsDisScore(\estimatedObservation_{\objPose_i,\sensingAction}, \estimatedObservation_{\objPose_j,\sensingAction})}{\sum_{\objPose \in \allObjStablePoses}\left(1-\obsDisScore(\estimatedObservation_{\objPose_i,\sensingAction}, \estimatedObservation_{\objPose,\sensingAction})\right)}
% \end{equation}


%compute the Baysian update
Our belief update rule is given by:

\begin{equation}\label{eq:beliefUdpate}
 \poseBeliefPerPose' = \beliefUpdateFunc\left({\poseBelief, \estimatedSensorFunc\left({ \objPose, \sensingAction}\right)}\right)= \beliefUpdateFunc\left({\poseBelief, \estimatedObservation_{\objPose,\sensingAction}}\right) 
\end{equation}

where for each $\objPose'\in\allObjStablePoses$ the update is Bayesian as follows:

\begin{equation}\label{eq:beliefUpdatee}
\transformedPoseBelief_{\objPose}(\objPose') = \frac{P(\estimatedObservation_{\objPose,\sensingAction}|\objPose')\cdot\poseBelief(\objPose')}{P(\estimatedObservation_{\objPose,\sensingAction})}  
\end{equation}

In our case $P(\estimatedObservation_{\objPose,\sensingAction}|\objPose') = \eta \cdot\obsSimScore(\estimatedObservation_{\objPose,\sensingAction}, \estimatedObservation_{\objPose',\sensingAction})$ such that $
\eta$ is a normalization factor to ensure that we have a valid distribution function. Also, according to the law of total probability: 
\begin{equation}
    P(\estimatedObservation_{\objPose,\sensingAction}) = \sum_{\objPose''\in\allObjStablePoses}P(\estimatedObservation_{\objPose,\sensingAction}|\objPose'')\cdot\poseBelief(\objPose'')
\end{equation}  

When we plug in that we get:

\begin{equation}\label{eq:beliefUpdatee0}
\poseBelief'_{\objPose}(\objPose') = \frac{\eta \cdot\obsSimScore(\estimatedObservation_{\objPose,\sensingAction}, \estimatedObservation_{\objPose',\sensingAction})\cdot\poseBelief(\objPose')}{\sum_{\objPose''\in\allObjStablePoses}\eta\cdot\obsSimScore(\estimatedObservation_{\objPose,\sensingAction}, \estimatedObservation_{\objPose'',\sensingAction})\cdot\poseBelief(\objPose'')}  
\end{equation}

the normalization factor can be canceled out, and we will be left with:

\begin{equation}\label{eq:beliefUpdatee1}
\poseBelief'_{\objPose}(\objPose') = \frac{\obsSimScore(\estimatedObservation_{\objPose,\sensingAction}, \estimatedObservation_{\objPose',\sensingAction})\cdot\poseBelief(\objPose')}{\mathbb{E}_{\objPose'' \sim \poseBelief}[\obsSimScore(\estimatedObservation_{\objPose,\sensingAction}, \estimatedObservation_{\objPose'',\sensingAction})]}  
\end{equation}

The updated belief is a valid distribution function: $$\sum_{\objPose'\in\allObjStablePoses}\poseBelief'_{\objPose}(\objPose') = \sum_{\objPose'\in\allObjStablePoses}\left(\frac{\obsSimScore(\estimatedObservation_{\objPose,\sensingAction}, \estimatedObservation_{\objPose',\sensingAction})\cdot\poseBelief(\objPose')}{\mathbb{E}_{\objPose'' \sim \poseBelief}[\obsSimScore(\estimatedObservation_{\objPose,\sensingAction}, \estimatedObservation_{\objPose'',\sensingAction})]}\right)=$$

$$= \frac{1}{\mathbb{E}_{\objPose'' \sim \poseBelief}[\obsSimScore(\estimatedObservation_{\objPose,\sensingAction}, \estimatedObservation_{\objPose'',\sensingAction})]}\cdot\sum_{\objPose'\in\allObjStablePoses}\obsSimScore(\estimatedObservation_{\objPose,\sensingAction}, \estimatedObservation_{\objPose',\sensingAction})\cdot\poseBelief(\objPose')=$$

$$= \frac{\mathbb{E}_{\objPose' \sim \poseBelief}[\obsSimScore(\estimatedObservation_{\objPose,\sensingAction}, \estimatedObservation_{\objPose',\sensingAction})]}{\mathbb{E}_{\objPose'' \sim \poseBelief}[\obsSimScore(\estimatedObservation_{\objPose,\sensingAction}, \estimatedObservation_{\objPose'',\sensingAction})]} = 1$$

Notice that $\poseBelief'_{\objPose}(\objPose') \propto \obsSimScore(\estimatedObservation_{\objPose,\sensingAction}, \estimatedObservation_{\objPose',\sensingAction})$ as expected.
%\fi

Our belief update rule is given by:

\begin{equation}\label{eq:beliefUdpate}
 \poseBeliefPerPose' = \beliefUpdateFunc\left({\poseBelief, \estimatedSensorFunc\left({ \objPose, \sensingAction}\right)}\right)= \beliefUpdateFunc\left({\poseBelief, \estimatedObservation_{\objPose,\sensingAction}}\right) 
\end{equation}

where for each $\objPose'\in\allObjStablePoses$ the update is Bayesian as follows:

\begin{equation}\label{eq:beliefUpdatee}
\transformedPoseBelief_{\objPose}(\objPose') = \frac{P(\estimatedObservation_{\objPose,\sensingAction}|\objPose')\cdot\poseBelief(\objPose')}{P(\estimatedObservation_{\objPose,\sensingAction})}  
\end{equation}



When we plug in that we get:

\begin{equation}\label{eq:beliefUpdatee0}
\poseBelief'_{\objPose}(\objPose') = \frac{\eta \cdot\obsSimScore(\estimatedObservation_{\objPose,\sensingAction}, \estimatedObservation_{\objPose',\sensingAction})\cdot\poseBelief(\objPose')}{\sum_{\objPose''\in\allObjStablePoses}\eta\cdot\obsSimScore(\estimatedObservation_{\objPose,\sensingAction}, \estimatedObservation_{\objPose'',\sensingAction})\cdot\poseBelief(\objPose'')}  
\end{equation}

the normalization factor can be canceled out, and we will be left with:

\begin{equation}\label{eq:beliefUpdatee1}
\poseBelief'_{\objPose}(\objPose') = \frac{\obsSimScore(\estimatedObservation_{\objPose,\sensingAction}, \estimatedObservation_{\objPose',\sensingAction})\cdot\poseBelief(\objPose')}{\mathbb{E}_{\objPose'' \sim \poseBelief}[\obsSimScore(\estimatedObservation_{\objPose,\sensingAction}, \estimatedObservation_{\objPose'',\sensingAction})]}  
\end{equation}

The updated belief is a valid distribution function: $$\sum_{\objPose'\in\allObjStablePoses}\poseBelief'_{\objPose}(\objPose') = \sum_{\objPose'\in\allObjStablePoses}\left(\frac{\obsSimScore(\estimatedObservation_{\objPose,\sensingAction}, \estimatedObservation_{\objPose',\sensingAction})\cdot\poseBelief(\objPose')}{\mathbb{E}_{\objPose'' \sim \poseBelief}[\obsSimScore(\estimatedObservation_{\objPose,\sensingAction}, \estimatedObservation_{\objPose'',\sensingAction})]}\right)=$$

$$= \frac{1}{\mathbb{E}_{\objPose'' \sim \poseBelief}[\obsSimScore(\estimatedObservation_{\objPose,\sensingAction}, \estimatedObservation_{\objPose'',\sensingAction})]}\cdot\sum_{\objPose'\in\allObjStablePoses}\obsSimScore(\estimatedObservation_{\objPose,\sensingAction}, \estimatedObservation_{\objPose',\sensingAction})\cdot\poseBelief(\objPose')=$$

$$= \frac{\mathbb{E}_{\objPose' \sim \poseBelief}[\obsSimScore(\estimatedObservation_{\objPose,\sensingAction}, \estimatedObservation_{\objPose',\sensingAction})]}{\mathbb{E}_{\objPose'' \sim \poseBelief}[\obsSimScore(\estimatedObservation_{\objPose,\sensingAction}, \estimatedObservation_{\objPose'',\sensingAction})]} = 1$$

Notice that $\poseBelief'_{\objPose}(\objPose') \propto \obsSimScore(\estimatedObservation_{\objPose,\sensingAction}, \estimatedObservation_{\objPose',\sensingAction})$ as expected.
%\fi
